# Supplementary material for: DualPrim: Compact 3D Reconstruction with Positive and Negative Primitives
Source: arXiv:2603.16133 source file (2026-03-17)
Supplement: Supplementary file 1 [file supp_comparison_cvpr2026.tex]

\newcommand{\suppImgWidth}{0.10}
\setlength{\tabcolsep}{10pt}

% --------------------------------------------------
% Macro for one image
% --------------------------------------------------
% \newcommand{\itwimg}[1]{\includegraphics[width=\itwImgWidth\textwidth]{#1}}
\newcommand{\suppImg}[2][]{%
  \vbox{%
    \hbox{\includegraphics[width=\suppImgWidth\textwidth]{figures/shapenet/#2}}%
    \ifx &#1&%
      % do nothing if #1 is empty
    \else
      % \vskip 1mm
      \hbox to \suppImgWidth\textwidth{\hss\small #1\hss}%
    \fi
  }%
}
% --------------------------------------------------
% Macro for one object (two rows)
% args:
% 1 object folder name
% 2 object name prefix
% 3 view id
% --------------------------------------------------
\newcommand{\tworowobjsupp}[2]{

% ---- first row ----
\suppImg[Input]{#1_input.png} &
\suppImg[Ours]{#2_#1_ours.png} &
\suppImg[PA~\cite{ye2025primitiveanything}]{#2_#1_pa.png} &
\suppImg[MA~\cite{chen2024meshanything}]{#2_#1_ma.png} &
\suppImg[MP~\cite{Liu2023marching}]{#2_#1_mp.png} &
\suppImg[EMS~\cite{liu2022EMS}]{#2_#1_ems.png} &
\suppImg[NVD~\cite{Munkberg_2022_CVPR}]{#2_#1_nvdiffrec.png}
\\

% ---- second row ----
\suppImg[FC~\cite{shen2023flexicubes}]{#2_#1_flexicube.png} &
\suppImg[RNS~\cite{rnbneus}]{#2_#1_neus2.png} &
\suppImg[{CAPRI}~\cite{yu2022capri}]{#2_#1_capri.png} &
\suppImg[{D$^{2}$CSG}~\cite{yu2023d}]{#2_#1_d2csg.png} &
\suppImg[{DiffCSG}~\cite{yuan2024diffcsg}]{#2_#1_diffcsg.png} &
\suppImg[2DGS~\cite{huang20242dgs}+MC]{#2_#1_2dgs_mc.png} &
\suppImg[2DGS~\cite{huang20242dgs}+CSG~\cite{yu2022capri}]{#2_#1_2dgs_csg.png}
\vspace{-1mm} \\[2pt]
}

\begin{figure*}[t]
\centering

\begin{tabular}{c c c c c c c}

% --------------------------------------------------
% Objects
% --------------------------------------------------

\tworowobjsupp{12f3fb99c95c6a7357891d676f728bc0}{airplane}
\vspace{-3mm}
\tworowobjsupp{10cfa696ba2259ccbbba142d6df53ce}{bench}
\vspace{-3mm}
\tworowobjsupp{2d1aa4e124c0dd5bf937e5c6aa3f9597}{bottle}
\vspace{-3mm}
\tworowobjsupp{1db4071178f5818250da8b99982a3057}{faucet}
\vspace{-3mm}
\tworowobjsupp{2b326c82b14dcdcfaf0affed7cfb91de}{clock}
\vspace{-3mm}
\tworowobjsupp{13e1e13465fa1a67b362845c6edb57fc}{faucet}

\end{tabular}

\caption{
Qualitative comparison on ShapeNet objects (part 1).
Each object occupies two rows.
The first row shows input, Ours, PA, MA, MP, EMS, and NVD.
The second row shows FC, RNS, CAPRI, D$^{2}$CSG, DiffCSG, 2DGS+MC, and 2DGS+CSG.
}
\label{fig:supp_comparison_cvpr2026_1}
\end{figure*}

\begin{figure*}[t]
\centering

\begin{tabular}{c c c c c c c}

% --------------------------------------------------
% Objects
% --------------------------------------------------

\tworowobjsupp{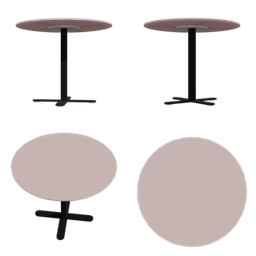}{table}
\vspace{-3mm}
\tworowobjsupp{1309cb5bbd90c7b250da8b99982a3057}{faucet}
\vspace{-3mm}
\tworowobjsupp{5b39e6a8f57199409bda39e34f423da8}{bookshelf}
\vspace{-3mm}
\tworowobjsupp{15e38eb29fb84898e7e684d25d4dcaf0}{lamp}
\vspace{-3mm}
\tworowobjsupp{18a9c13c3999e9c186abe5555a3b447d}{table}
\end{tabular}

\caption{
Qualitative comparison on ShapeNet objects (part 2).
Each object occupies two rows.
The first row shows input, Ours, PA, MA, MP, EMS, and NVD.
The second row shows FC, RNS, CAPRI, D$^{2}$CSG, DiffCSG, 2DGS+MC, and 2DGS+CSG.
}
\label{fig:supp_comparison_cvpr2026_2}
\end{figure*}
